# Supplementary material for: Sparse Recovery with Graph Constraints
Source: arXiv:1207.2829 source file (2013-03-09)
Supplement: Supplementary file 1 [file appendix.tex]

\appendix

\subsection{Proof of Theorem \ref{thm:random}}

%\begin{proof}[of Theorem \ref{thm:random}]
%We know that $k$-sparse vectors can always be identified if and only
%if every $2k$ columns of the measurement matrix is linearly
%independent. Let $m$ denote the number of measurements.
Let $A^{m
\times n}$ denote the  matrix with $m$ realizations
of the $n$-step Markov chain. To prove the statement, from \cite{CaT05}, we only need
to show that  % if $m=O(g(k) \log n)$ for some function $g$, then the probability that the measurement matrix
the probability that every $2k$ columns of $A$ are linearly independent goes to 1
as $n$ goes to infinity.

%We first characterize the probability that $2k$ given columns are
%linearly dependent.
%Let $I$ be a set of $2k$ different indices,
%then
Let $A_I$ be a submatrix of $A$ with columns in $I$, where $I$ is an index set with $|I|=2k$.
%Let $P_d^I$ denote the probability that rank($A_I$)$<2k$. %$A_I$ has
%$\lfloor \frac{m}{2k}\rfloor$ number of $2k$ by $2k$ submatrices
%where
Let $A_{S_jI}$ ($1\leq j \leq \lfloor \frac{m}{2k}\rfloor$) be a
submatrix of $A_I$ formed by row $2k(j-1)+1$ to row $2kj$ of $A_I$.
Given $I$, the probability that rank($A_{S_jI}$)$<2k$
is the same for every given $j$, and let it denoted by $\pi _d^I$.
Let $P_d^I$ denote the probability that rank($A_I$)$<2k$, then % and let $\pi _d^I$ denote the probability that rank($A_{S_jI}$)$<2k$
%for given $j$. Note that given $I$, $\pi _d^I$ is the same for every
%matrix
%$A_{S_jI}$, $\forall j$. % ($1 \leq j \leq \lfloor \frac{m}{2k}\rfloor$).
%Note that rank($A_I$)$< 2k$ implies that rank($A_{S_jI}$)$<2k$ for each
%such matrix $A_{S_jI}$, then %and each measurement corresponds to an
%independent realization of Markov chain, then we have
\begin{equation}\label{eqn:pdi}
P_d^I \leq (\pi _d^I)^{\lfloor \frac{m}{2k}\rfloor}.
\end{equation}

To characterize $\pi _d^I$,
 consider matrix $B^{2k \times 2k}$ with $B_{ii}=0$ for
$i=2,3,...,2k$ and $B_{ij}=1$ for all the other elements.
Since rank($B$)$=2k$, then % Then given $j$, if matrix
%$A_{S_jI}$ has the same rows as $B$, then $A_{S_jI}$ is full rank.
%Thus,
\begin{equation}\label{eqn:pidi}
\pi_d^I \leq 1- P(A_{S_jI} \textrm{ is a row permutation of } B).
\end{equation}
%Since the transition matrix
%%\begin{equation}
%$P =\left[ {\begin{array}{*{20}c}
%   0 & 1  \\
%   {0.5} & {0.5}  \\
%\end{array}} \right]$, %=VDV^{-1},
%\end{equation}
%where $V= \left[ {\begin{array}{*{20}c}
%   -\frac{2\sqrt{5}}{5} & -\frac{\sqrt{2}}{2}  \\
%   \frac{\sqrt{5}}{5} & -\frac{\sqrt{2}}{2}  \\
%\end{array}} \right]$ and $D= \left[ {\begin{array}{*{20}c}
%   -\frac{1}{2} & 0  \\
%   0 & 1 \\
%\end{array}} \right]$,
%then for an integer $r \geq 1$,
%\begin{eqnarray}
%P^r&=&VD^rV^{-1} \nonumber\\
%&=&\left[ {\begin{array}{*{20}c}
%   -\frac{2\sqrt{5}}{5} & -\frac{\sqrt{2}}{2}  \\
%   \frac{\sqrt{5}}{5} & -\frac{\sqrt{2}}{2}  \\
%\end{array}} \right] \left[ {\begin{array}{*{20}c}
%   \frac{(-1)^r}{2^r} & 0  \\
%   0 & 1 \\
%\end{array}} \right]\left[ {\begin{array}{*{20}c}
%   -\frac{\sqrt{5}}{3} & \frac{\sqrt{5}}{3}  \\
%   -\frac{\sqrt{2}}{3} & -\frac{2\sqrt{2}}{3}  \\
%\end{array}} \right] \nonumber \\
%&=& \left[ {\begin{array}{*{20}c}
%   \frac{2}{3}(-\frac{1}{2})^r+\frac{1}{3} & -\frac{2}{3}(-\frac{1}{2})^r+\frac{2}{3}  \\
%   -\frac{1}{3}(-\frac{1}{2})^r+\frac{1}{3} & \frac{1}{3}(-\frac{1}{2})^r+\frac{2}{3}  \\
%\end{array}} \right].
%\end{eqnarray}
%Therefore,
One can check that in this Markov chain, for every $ 1 \leq i < k \leq n$, $P(X_k=1~|~X_i=1) \geq 1/2$, $P(X_k=0~|~X_i=1)\geq 1/4$, $P(X_k=1~|~X_i=0) \geq 1/2$,
%\begin{equation}
%P(X_k=1|X_i=1)=\frac{1}{3}(-\frac{1}{2})^{k-i}+\frac{2}{3} \geq
%\frac{1}{2},
%\end{equation}
%\begin{equation}
%P(X_k=0|X_i=1)=-\frac{1}{3}(-\frac{1}{2})^{k-i}+\frac{1}{3} \geq
%\frac{1}{4},
%\end{equation}
%and
%\begin{equation}
%P(X_k=1|X_i=0)=-\frac{2}{3}(-\frac{1}{2})^{k-i}+\frac{2}{3} \geq
%\frac{1}{2}.
%\end{equation}
%Since $X_1=1$, %$P(X_1=1)=1$ and $P(X_1=0)=0$, then
%for every $1 \leq k \leq n$,
and $P(X_k=1)\geq 1/2$. % by simple calculation.
%\begin{eqnarray}
%P(X_k=1)&=&P(X_1=1)P(X_k=1|X_1=1) \nonumber
%\\
%&&+P(X_1=0)P(X_k=1|X_1=1) \nonumber
%\\
%&=& \frac{1}{3}(-\frac{1}{2})^{k-1}+\frac{2}{3} \nonumber \\&\geq&
%\frac{1}{2}.
%\end{eqnarray}
%Then one can calculate that %the probability that $A_{S_jI}$ is equal to $B$ is
%\begin{eqnarray}
%P(A_{S_jI}=B)&\geq&
%(\frac{1}{2}\cdot(\frac{1}{2})^{2k-1})\cdot(\frac{1}{2}\cdot
%\frac{1}{4}\cdot (\frac{1}{2})^{2k-2})^{2k-1} \nonumber
%\\
%&=&(\frac{1}{2})^{4k^2+2k-1}.
%\end{eqnarray}
%$P(A_{S_jI}=B)\geq (1/2)^{4k^2+2k-1}$ for all $I$.
Since $B$ has $(2k)!$ different row permutations, %one can calculate that % matrices that have the same rows as $B$,
%then
\begin{equation}\label{eqn:pab}
%\hspace{-0.05in}
P(A_{S_jI} \textrm{ is a row permutation of } B)\geq
(2k)!/2^{4k^2+2k-1}.
\end{equation}
Combining (\ref{eqn:pdi}), (\ref{eqn:pidi}) and (\ref{eqn:pab}), we
have
%\begin{equation}
%P_d^I \leq
%(1-(2k)!(\frac{1}{2})^{4k^2+2k-1})^{\lfloor\frac{m}{2k}\rfloor} \leq
%e^{-(2k)!(\frac{1}{2})^{4k^2+2k-1}\lfloor\frac{m}{2k}\rfloor}.
%\end{equation}
%Then
\begin{align}
&P(\textrm{every } 2k \textrm{ columns of } A \textrm{ are
linearly independent}) \nonumber \\
=&1-P(\textrm{rank}(A_I)<2k \textrm{ for some } I \textrm { with }
|I|=2k) \nonumber \\
\geq & 1-{n\choose2k}P_d^I  \geq
1-{n\choose2k}e^{-(2k)!(\frac{1}{2})^{4k^2+2k-1}\lfloor\frac{m}{2k}\rfloor}, \nonumber %\label{eqn:pind}
\end{align}
where the first inequality follows from the union bound. Then if
$m=g(k) \log n= (2k+1)2^{4k^2+2k-1}\log n /(2k-1)!$,
%from (\ref{eqn:pind}) we have
the probability that every $2k$ columns of $A$ are linearly
independent is at least $1-1/((2k)!n)$.
%\begin{equation}
%P(\textrm{every } 2k \textrm{ columns of } A \textrm{ are linearly
%independent}) \geq 1-\frac{1}{(2k)!n}.
%\end{equation}
%Therefore, with high probability % at least $1-\frac{1}{(2k)!n}$,
%$O(g(k)\log n)$ measurements generated by the Markov chain are
%sufficient to identify $k$-sparse vectors.
%Then the statement follows.
\subsection{Proof of Proposition \ref{thm:ring4gt}}

%\begin{proof}
%Consider the number of measurements needed to locate
%Suppose two non-zero elements are on nodes
%$2i-1$ and $2i$ for some $1\leq i \leq \lfloor \frac{n}{2}\rfloor$.
%by group testing if we know that these two non-zero elements happen.
%Clearly this number is no greater
%than the number of measurements needed to locate two general non-zero elements associated with $\mathcal{G}^4$.
We view nodes $2i-1$ and $2i$ as a group for every $i$ ($1
\leq i \leq \lfloor \frac{n}{2}\rfloor$), denoted by $B_i$. Consider the special case that for some $t$, both nodes in $B_t$ are `1's, and all other nodes are `0's. % then
%there are $\lfloor \frac{n}{2}\rfloor$ groups in total.
%If both nodes in $B_j$ are `1's for some $j$,
Then every measurement that
passes either node or both nodes in $B_t$ is always `1'.  %no matter which
%node/nodes the measurement passes in the group testing setup.
Consider a reduced graph with
$B_i$, $\forall i$ %($1 \leq i \leq \lfloor \frac{n}{2}\rfloor$)
as nodes, and
   edge $(B_i,B_j)$ ($i \neq j$) exists only if in $\mathcal{G}^4$ there is a path from a node in $B_i$ to a node in $B_j$
without going though any other node not in $B_i$ or $B_j$. %in $B_k$ for some $k$ with $k
%\neq i$ and $k \neq j$. Then
$B_i$ is `1' if both node $2i-1$ and node $2i$ in $\mathcal{G}^4$ are `1's and is `0' otherwise.
The reduced network is a ring with $\lfloor \frac{n}{2}\rfloor$ nodes, %.each
%node $B_i$ connecting to $B_{i-1 (\textrm{mod }n)}$ and $B_{i+1
%(\textrm{mod }n)}$.  Since $\lceil n/2\rceil$ measurements are
%necessary to locate one non-zero element in an $n$-node ring network, then we
%need
and thus $\lfloor n/4 \rfloor$ measurements are required to locate one
non-zero element in the reduced network. %two errors on nodes $2i-1$ and $2i$
%for some $1\leq i \leq \lfloor \frac{n}{2}\rfloor$.
Then only to locate two consecutive non-zero elements associated with $\mathcal{G}^4$,  we need at least $\lfloor n/4 \rfloor$ measurements, and the claim follows.
 %and thus, $\lfloor n/4 \rfloor$ is also a lower bound for locating two general non-zero elements.
%\end{proof}
\subsection{Proof of Theorem \ref{thm:np}}

%\begin{proof}[Proposition \ref{thm:np}]
%Given disjoint sets $S_1$,...,$S_r$ with $
%\cup_i S_i = V$,
Since checking whether or not $r$ given sets %$S_1$,...,$S_r$
form an $r$-partition takes polynomial time, $r$-partition problem is NP.
%For each $S_i$, we check whether or
%not $V \backslash S_i$ is connected in $O(|V|+|E|)$ time. And it takes
%$O(|V|+|E|)$ time to check whether or not every node has a neighbor
%that is not in the same set.

We   next show %the $r$-partition problem is NP-complete for $r \geq 3$ by proving
that %if $r\geq 3$,
the NP-complete $r$-coloring ($r \geq 3$) problem
is polynomial time reducible to
$r$-partition problem.

Let $G = (V,E)$ and an integer $r$ be an instance of
$r$-coloring. For every $(u, v) \in E$, add a node
$w$ and two edges $(w,u)$ and $(w, v)$. Let $W$ denote the set of nodes added. Add a edge between every pair of nodes in $V$
not already joined by a edge. Let $H$ denote the augmented graph and let %$V'$ denote the set of nodes in $H$. Then
$V'=V \cup W$. %Note that $V'=V \cup W$, and $H_V$ is a complete graph. %Consider the problem of
%finding a $r$-partition of $H$.
We claim that if there exists an $r$-partition of $H$, then we can obtain an $r$-coloring of $G$, and vice versa. %conversely, if there exists an $r$-coloring of $G$, then we can obtain an $r$-partition of $H$.

Let $S_i$ ($i=1,...,r$) be an $r$-partition of $H$. %We will find a $r$-coloring of $G$.
%Note that for every $(u, v) \in E$,  $u$ and $v$ cannot belong to the same set $S_i$ for any $i$. %To see this,
Suppose there exists edge $(u, v) \in E$ s.t. $u$ and $v$ both belong to $S_i$ for some $i$. Let $w$ denote the node in $W$ that only directly connects to $u$ and $v$. If $w \in S_i$, then $w$ has both neighbors in the same set with $w$, contradicting the definition of $r$-partition. If $w \notin S_i$, then $H_{V'\backslash S_i}$ is disconnected since $w$ does not connect to any node in $V'\backslash S_i$. It also contradicts the definition of $r$-partition. Thus, for every $(u,v) \in E$, node $u$ and $v$ belong to two  sets $S_i$ and $S_j$ with $i \neq j$. %Now we can color the graph $G=(V,E)$ with $r$ colors such that nodes in the same set $S_i$ have the same color, and one can check that it is indeed
Then we obtain an $r$-coloring of $G$.

%If there exists an $r$-coloring of $G$ and
Let $C_i \subset V$ ($i=1,...,r$) denote an $r$-coloring of $G$. %the set of nodes that are colored with $i$th color.
We claim that $N_i=C_i$ ($i=1, ..., r-1$), and $N_r=C_r \cup W$ form an $r$-partition of $H$. %To see this,
First note for every $u \in V$, at least one of its neighbors is not in the same set as $u$. % since $H_V$ is a complete subgraph. %, there is a edge $(i, j)$ between every two different nodes $i$ and $j$ in $V$,  then for every node $u$ in $V$, at least one of its neighbors is not in the same set as $u$.
For every  $w \in W$, $w$ is directly connected to $u$ and $v$ for some $(u,v) \in E$, %From the definition of $r$-coloring, %$u$ and $v$ are colored with different colors, i.e.
and $u$ and $v$ are in different sets $C_i$ and $C_j$ for some $i \neq j$. Therefore, $w$ has at least one neighbor that is not in $N_r$. Second, we will show $H_{V' \backslash N_i}$ is connected for all $i$. $H_{V' \backslash N_r}$ is  a complete subgraph, and thus connected.
For every $i<r$, let $S_i:=V \backslash C_i$, then $V' \backslash N_i= S_i \cup W$. $H_{S_i}$ is a complete subgraph, and thus connected. For every $w  \in W$, since its two neighbors cannot be both in $C_i$, then at least one neighbor belongs to $S_i$, %thus $w$ is directly connected to some node in $S_i$. Therefore,
thus $H_{V' \backslash N_r}=H_{S_i \cup W}$ is connected. $N_i$ ($i=1,..., r$) thus forms an $r$-partition.
%
%Since $r$-coloring problem is reducible to
%$r$-partition problem and
%Since $r$-coloring is NP-complete for $r\geq3$, thus $r$-partition problem is also NP-complete for $r \geq 3$.
%\end{proof} 
